# Supplementary material for: Weakly Supervised Volumetric Image Segmentation with Deformed Templates
Source: arXiv:2106.03987 source file (2022-06-03)
Supplement: Supplementary file 1 [file Appendix.pdf]

## 6 Appendix

### 6.1 Training and Hyper-parameter tuning

Experiments were conducted on 3 NVIDIA Tesla V100 GPUs. Each model was optimized using Adam [20] optimizer with a learning rate of  $10^{-4}$  for 150000 iterations. Due to the large number of experiments required to generate the plots in Fig. 7, 8, 9, only one instance of each experiment was conducted. For Table 1, each experiment was repeated 3 times.

Hyper-parameter ( $\lambda$  and  $\gamma$ ) tuning were done using the validation set of the Hippocampus dataset. As mentioned in section 4.1, same hyper-parameters were used for all three dataset because the hyper-parameters from the hippocampus dataset were sufficient to demonstrate the effectiveness of the proposed method in the other two datasets as well.

### 6.2 More Qualitative Results

We show more qualitative results in Fig. 11 which further demonstrate the effectiveness of our approach. Here, the results are shown from the experiments that use the minimum amount of annotation for baseline and **T-Net**. For the baseline method it is 1 slice per sample and for **T-Net** it is 25 points per sample.

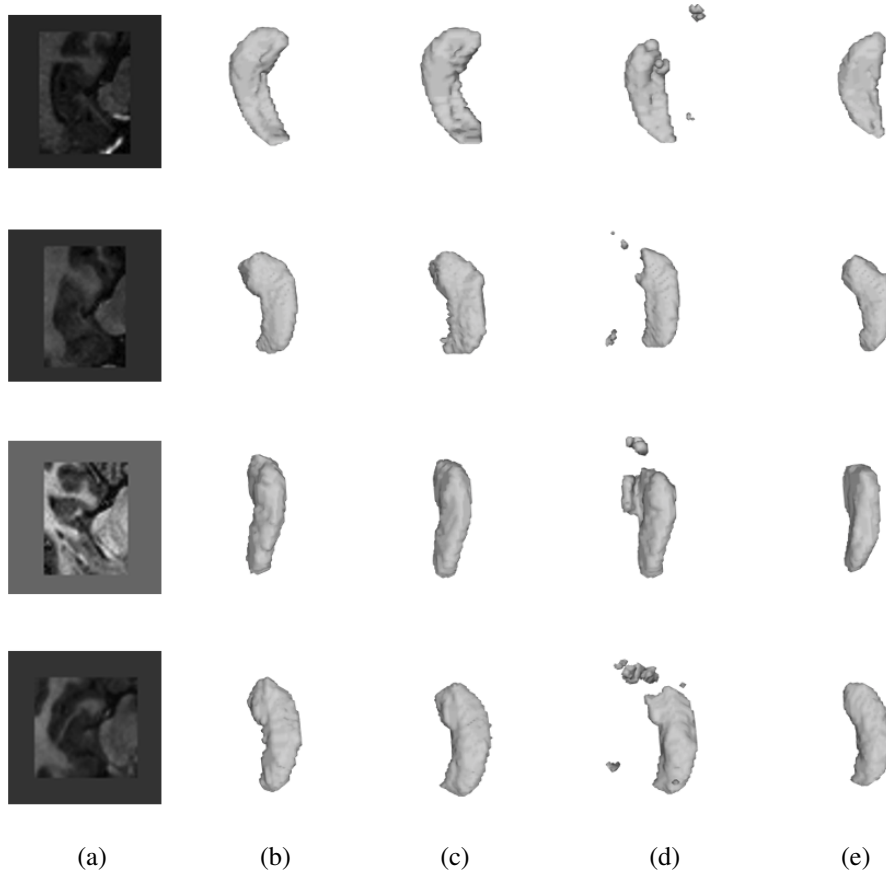

Figure 11: Results. (a) A slice from the input volume from top to bottom (b) Ground truth (c) U-Net with full-supervision (d) Baseline (e) **T-Net**.

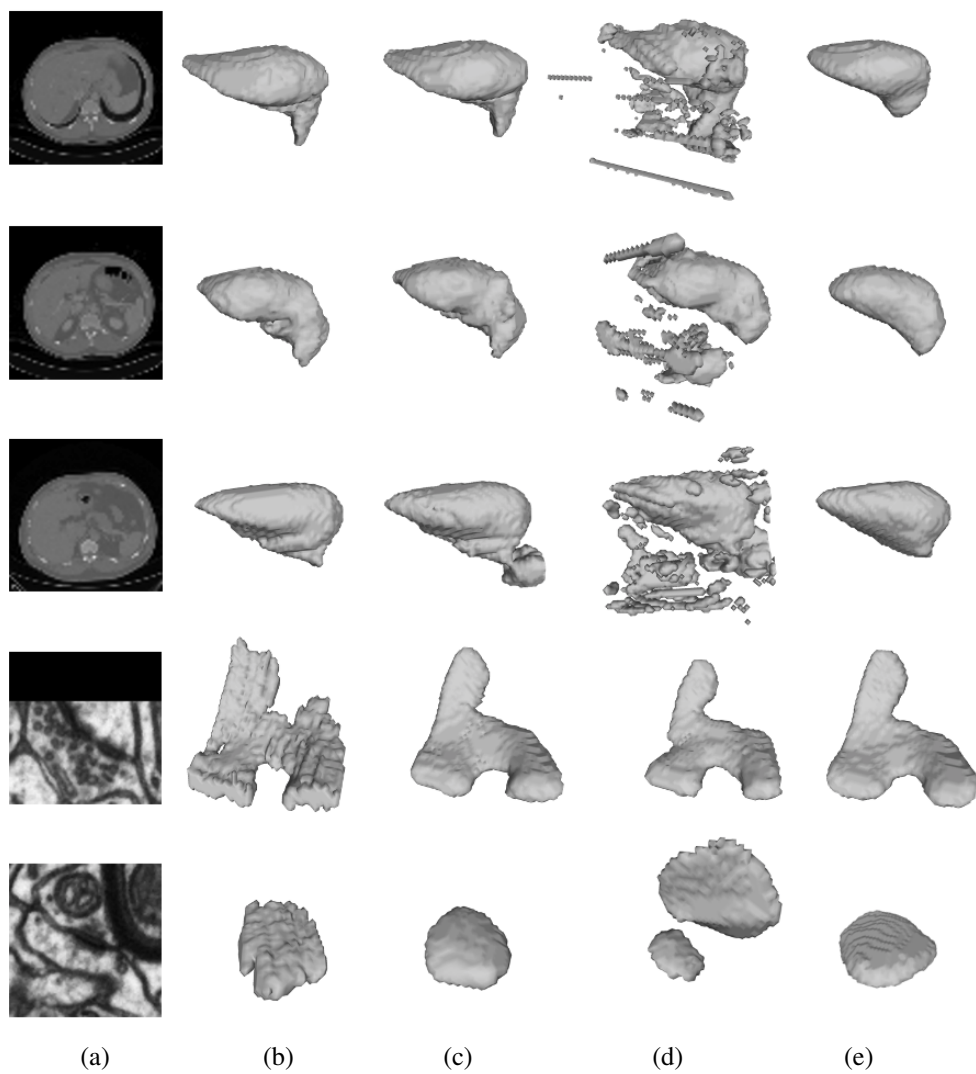

Figure 11: Results (Cont.). (a) A slice from the input volume from top to bottom (b) Ground truth (c) U-Net with full-supervision (d) Baseline (e) **T-Net**.

## References

- [1] D. Akuna, H. Ling, A. Kar, and S. Fidler. Efficient Interactive Annotation of Segmentation Datasets with Polygon-RNN++. In *Conference on Computer Vision and Pattern Recognition*, 2018.
- [2] A. Bearman and O. Russakovsky, V. Ferrari, and L. Fei-Fei. What’s the point: Semantic segmentation with point supervision. In *ECCV*, 2016.
- [3] G. Bertasius, H. S. Park, S. X. Yu, and J. Shi. Unsupervised Learning of Important Objects from First-Person Videos. In *International Conference on Computer Vision*, 2017.
- [4] Ö. Çiçek, A. Abdulkadir, S. Lienkamp, T. Brox, and O. Ronneberger. 3D U-Net: Learning Dense Volumetric Segmentation from Sparse Annotation. In *Conference on Medical Image Computing and Computer Assisted Intervention*, pages 424–432, 2016.
- [5] D. Cremers, S. Osher, and S. Soatto. Kernel Density Estimation and Intrinsic Alignment for Shape Priors in Level-Set Segmentation. *International Journal of Computer Vision*, 2006.
- [6] A. Dalca, E. Yu, P. Golland, B. Fischl, M. Sabuncu, and J. Iglesias. Unsupervised Deep Learning for Bayesian Brain MRI Segmentation. In *Conference on Medical Image Computing and Computer Assisted Intervention*, 2019.
- [7] R. Dorent, S. Joutard, J. Shapey, S. Bisdas, N. Kitchen, R. Bradford, S. Saeed, M. Modat, S. Ourselin, and T. Vercauteren. Scribble-based Domain Adaptation via Co-segmentation. In *Conference on Medical Image Computing and Computer Assisted Intervention*, 2020.
- [8] V. Duque, D. Chanti, M. Crouzier, A. Nordez, L. Lacourpaille, and D. Mateus. Spatio-temporal Consistency and Negative Label Transfer for 3D freehand US Segmentation. In *Conference on Medical Image Computing and Computer Assisted Intervention*, 2020.
- [9] T. Durand, T. Mordan, N. Thome, and M. Cord. Wildcat: Weakly supervised learning of deep convnets for image classification, pointwise localization and segmentation. In *CVPR*, 2017.
- [10] X. Feng, J. Yang, A. Laine, and E. Angelini. Discriminative Localization in CNNs for Weakly-Supervised Segmentation of Pulmonary Nodules. In *Conference on Medical Image Computing and Computer Assisted Intervention*, pages 568–576, 2017.
- [11] D. Freedman and T. Zhang. Interactive Graph-Cut Based Segmentation with Shape Priors. In *Conference on Computer Vision and Pattern Recognition*, pages 755–62, 2005.
- [12] W. Ge, S. Yanga, and Y. Yu. Multi-evidence filtering and fusion for multi-label classification, object detection and semantic segmentation based on weakly supervised learning. In *CVPR*, 2018.
- [13] W. Ge, X. Lin, and Y. Yu. Weakly supervised complementary parts models for fine-grained image classification from the bottom up. In *CVPR*, 2019.
- [14] C. Hsu, K. Hsu, C. Tsai, Y. Lin, and Y. Chuang. Weakly supervised instance segmentation using the bounding box tightness prior. In *NIPS*, 2019.
- [15] Z. Huang, X. Wang, J. Wang, W. Liu, and J. Wang. Weakly-supervised semantic segmentation network with deep seeded region growing. In *CVPR*, 2018.
- [16] M. Januszewski, J. Kornfeld, P. Li, A. Pope, T. Blakely, L. Lindsey, J. Maitin-Shepard, M. Tyka, W. Denk, and V. Jain. High-Precision Automated Reconstruction of Neurons with Flood-Filling Networks. *Nature Methods*, 2018.
- [17] M. Kass, A. Witkin, and D. Terzopoulos. Snakes: Active Contour Models. *International Journal of Computer Vision*, 1(4):321–331, 1988.
- [18] A. Kavur and M. Selver. CHAOS Challenge - Combined (CT-MR) Healthy Abdominal Organ Segmentation. In *arXiv Preprint*, 2020.
- [19] A. Khoreva, R. Benenson, J. Hosang, M. Hein, and B. Schiele. Simple Does It: Weakly Supervised Instance and Semantic Segmentation. In *Conference on Computer Vision and Pattern Recognition*, pages 1665–1674, 2017.
- [20] D. P. Kingma and J. Ba. Adam: A Method for Stochastic Optimization. In *International Conference on Learning Representations*, 2015.

- [21] V. Kulharia, S. Chandra, A. Agrawal, P. Torr, and A. Tyagi. Box2seg: Attention weighted loss and discriminative feature learning for weakly supervised segmentation. In *ECCV*, 2020.
- [22] M. Lee, K. Petersen, N. Pawlowski, B. Glocker, and Michiel Schaap. TETRIS: Template Transformer Networks for Image Segmentation With Shape Priors. In *IEEE Transactions on Medical Imaging*, 2019.
- [23] H. Ling, J. Gao, A. Kar, W. Chen, and S. Fidler. Fast Interactive Object Annotation with Curve-Gcn. In *Conference on Computer Vision and Pattern Recognition*, pages 5257–5266, 2019.
- [24] K. Maninis, S. Caelles, J. Pont-Tuset, and L. Gool. Deep extreme cut: From extreme points to object segmentation. In *CVPR*, 2018.
- [25] F. Milletari, N. Navab, and S.-A. Ahmadi. V-Net: Fully Convolutional Neural Networks for Volumetric Medical Image Segmentation. In *arXiv Preprint*, June 2016.
- [26] Zahra Mirikharaji and Ghassan Hamarneh. Star Shape Prior in Fully Convolutional Networks for Skin Lesion Segmentation. In *Conference on Medical Image Computing and Computer Assisted Intervention*, pages 737–745, 2018.
- [27] E.N. Mortensen and W.A. Barrett. Intelligent Scissors for Image Composition. In *ACM SIGGRAPH*, pages 191–198, August 1995.
- [28] S. Peng, W. Jiang, H. Pi, X. Li, H. Bao, and X. Zhou. Deep Snake for Real-Time Instance Segmentation. In *Conference on Computer Vision and Pattern Recognition*, 2020.
- [29] H. Qu, P. Wu, Q. Uuqang, J. Yi, Z. Yan, G. Riedlinger, S. De, S. Zhang, and D. Metaxas. Weakly Supervised Deep Nuclei Segmentation Using Partial Points Annotation in Histopathology Images. In *IEEE Transactions on Medical Imaging*, 2020.
- [30] H. Roth, L. Zhang, D. Yang, F. Milletari, Z. Xu, X. Wang, and D. Xu. Weakly supervised segmentation from extreme points. In *Conference on Medical Image Computing and Computer Assisted Intervention*, 2019.
- [31] A. Shvets, A. Rakhlin, A. Kalinin, and V. Iglovikov. Automatic Instrument Segmentation in Robot-Assisted Surgery Using Deep Learning. In *arXiv Preprint*, 2018.
- [32] C. Song, Yan Huang, Wanli Ouyang, and Liang Wang. Box-driven class-wise region masking and filling rate guided loss for weakly supervised semantic segmentation. In *CVPR*, 2019.
- [33] H. Spitzer, K. Amunts, S. Harmeling, and T. Dickscheid. Parcellation of Visual Cortex on High-Resolution Histological Brain Sections Using Convolutional Neural Networks. In *International Symposium on Biomedical Imaging*, pages 920–923, 2017.
- [34] H. Spitzer, K. Kiwitz, K. Amunts, S. Harmeling, and T. Dickscheid. Improving Cytoarchitectonic Segmentation of Human Brain Areas with Self-Supervised Siamese Networks. In *Conference on Medical Image Computing and Computer Assisted Intervention*, 2018.
- [35] Z. Wang, D. Acuna, H. Ling, A. Kar, and S. Fidler. Object Instance Annotation with Deep Extreme Level Set Evolution. In *European Conference on Computer Vision*, 2020.
- [36] U. Wickramasinghe, G. Knott, and P. Fua. Probabilistic atlases to enforce topological constraints. In *Conference on Medical Image Computing and Computer Assisted Intervention*, 2019.
- [37] U. Wickramasinghe, E. Remelli, G. Knott, and P. Fua. Vox2mesh: 3d mesh model generation from volumetric data. In *Conference on Medical Image Computing and Computer Assisted Intervention*, 2020.
- [38] U. Wickramasinghe, G. Knott, and P. Fua. Deep active surface models. In *Conference on Computer Vision and Pattern Recognition*, 2021.
- [39] L. Yang, Y. Wang, X. Xiong, J. Yang, and A. Katsaggelos. Efficient video object segmentation via network modulation. In *CVPR*, 2018.
- [40] T. Zhao and Z. Yin. Weakly Supervised Cell Segmentation by Point Annotation. In *IEEE Transactions on Medical Imaging*, 2020.
- [41] C. Zotti, Z. Luo, A. Lalande, and P. Jodoin. Convolutional Neural Network With Shape Prior Applied to Cardiac MRI Segmentation. In *IEEE Transactions on Medical Imaging*, 2019.
